# Supplementary material for: One-Shot Imitation under Mismatched Execution
Source: arXiv:2409.06615 source file (2025-03-28)
Supplement: Supplementary file 1 [file appendix.tex]

\appendix

\section{Appendix}

We report metrics associated with Fig 2 in Table~\ref{tab:success_rates} and run additional ablations to investigate the importance of segment lengths when performing retrievals. We additionally provide more details about our model architecture and implementation.

\begin{table}[h]
\centering

% \vspace{3pt}
% \renewcoand{\arraystretch}{1.1}
\resizebox{\textwidth}{!}{
\begin{tabular}{cc|ccc|cc}
\toprule
& Model $\xrightarrow{}$  & \multicolumn{1}{c}{\textsc{Baseline}} & \multicolumn{2}{c|}{\textsc{Ours}} & \multicolumn{1}{c}{\textsc{Gold Standard}}\\  
\cmidrule{3-3} \cmidrule{4-5} \cmidrule{6-6}
& Metric $\downarrow$ & \textsc{XSkill} & \textsc{RHyME-TCC} & \textsc{RHyME-OT} & \textsc{OraclePairing}\\ 
\midrule
\parbox[t]{2pt}{\multirow{2}{*}{\rotatebox[origin=c]{90}{\small{\textsc{Easy}}}}}
 & Task Recall & 82\% ($\pm$ 3.5) & 75\% ($\pm$ 1.7) &  96\% ($\pm$ 1.3) & 92\% ($\pm$ 2.7)\\
 & Task Imprecision & 5\% ($\pm$ 1.7) & 5\% ($\pm$ 1.7) &  5\% ($\pm$ 1.0) & 7\% ($\pm$ 2.3) \\
\midrule
\parbox[t]{2pt}{\multirow{2}{*}{\rotatebox[origin=c]{90}{\small{\textsc{Med.}}}}}
  & Task Recall & 40\% ($\pm$ 2.7) & 57\% ($\pm$ 4.2) &  72\% ($\pm$ 5.8) & 92\% ($\pm$ 2.9)\\
 & Task Imprecision & 2\% ($\pm$ 1.1) & 51\% ($\pm$ 3.4) &  4\% ($\pm$ 1.9) & 0\% ($\pm$ .00) \\
\midrule
\parbox[t]{2pt}{\multirow{2}{*}{\rotatebox[origin=c]{90}{\small{\textsc{Hard}}}}}
   & Task Recall & 1\% ($\pm$ 1.2) & 34\% ($\pm$ 4.2) &  53\% ($\pm$ 5.5) & 92\% ($\pm$ 2.2)\\
 & Task Imprecision & 53\% ($\pm$ 5.2) & 65\% ($\pm$ 4.5) &  28\% ($\pm$ 5.1) & 1\% ($\pm$ 1.1) \\

% \midrule
% \hline
\bottomrule

\end{tabular}
}

\vspace{3pt}
\caption{\small{We report exact metrics and standard errors for the bar plots in Fig~\ref{fig:dataset_barplot}}.}

\label{tab:success_rates}
\vspace{-5mm}
\end{table}

\subsection{Segment Length for Retrievals}

In this section, we vary the segment length $K$ from Algorithm 2 for RHyME-OT on the Sphere-Hard dataset and report Task Recall and Task Imprecision results in Table~\ref{tab:seg_length}. Instead of a constant $K$ for all videos, we deploy $K$ as a function of the video length: that is, for a sequence of $T$ images, $K = \frac{T}{K'}$ where $K'$ is the total number of short horizon segments we split the video into. Increasing $K'$ yields more demonstrator clip retrievals. We qualitatively find that the synthesized videos with lower $K'$ often only consist of a strict subset of tasks from the original robot demonstration (thus yielding the highest task imprecision when $K'=1$), while those from higher $K'$ are more likely to accurately capture all the tasks in the robot demonstration. For our results throughout the paper, we simply select $K' = 2$, but we show that as long as the segment lengths are not too long (i.e. $K'$ is not too small), Optimal Transport retrievals provide similar results regardless of segment length. While higher values of $K'$ may lead to the construction of demonstrations with redundant tasks, the Transformer-based Skill Alignment Transformer described in Section~\ref{sec:model_arch} is able to learn relations between the robot's current state and the tasks in the entire demonstration video to extract the most relevant task embedding for the policy.

\begin{table}[h]
\centering

% \vspace{3pt}
% \renewcoand{\arraystretch}{1.1}
\resizebox{\textwidth}{!}{
\begin{tabular}{cc|cccc|c}
\toprule
& Video Splits $K'$ $\xrightarrow{}$  & \multicolumn{4}{c|}{\textsc{RHyME-OT}} \\  
\cmidrule{3-3} \cmidrule{4-6} \cmidrule{7-7}
& Metric $\downarrow$ & $K'=1$ & $K'=2$ & $K'=3$ & $K'=4$ \\ 
\midrule
\parbox[t]{2pt}{\multirow{2}{*}{\rotatebox[origin=c]{90}{\small{\textsc{Hard}}}}}
   & Task Recall & 49\% ($\pm$ 2.9) & 53\% ($\pm$ 3.6) & 58\% ($\pm$ 4.5) & 53\% ($\pm$ 2.6)\\
 & Task Imprecision & 28\% ($\pm$ 4.2) & 21\% ($\pm$ 3.7) & $\tbcolorg$ 12\% ($\pm$ 3.8) & 14\% ($\pm$ 3.7) \\

% \midrule
% \hline
\bottomrule

\end{tabular}
}

\vspace{3pt}
\caption{\small{We report Task Recall and Task Imprecision rates when varying the number of short horizon segments $K'$ we divide each long-horizon robot demonstration into to perform retrievals with RHyME-OT on the Sphere-Hard dataset}}.

\label{tab:seg_length}
\vspace{-5mm}
\end{table}

\subsection{Representation Alignment \label{sec:rep_align}}
\vspace{-12mm}
We utilize common representation alignment methods~\cite{Sermanet2017TimeContrastiveNS, Nair2022R3MAU, Oord2018RepresentationLW, caron2020unsupervised, xu2023xskill} to train our vision encoder $\phi$ that is used to produce image embeddings from videos, and describe them briefly.

\textbf{Temporal Alignment.} This alignment method leverages that image frames temporally close in a video are likely to be similar. We utilize the Time Contrastive Loss, used extensively in learning representations for robotics~\cite{Sermanet2017TimeContrastiveNS, Nair2022R3MAU}. For an image embedding at timestep $t$, $z^t$, we define a positive set $\mathbf{z^{+}} = \{z^{t'}, |t'-t| \leq w\}$  and negative set $\mathbf{z^{-}} = \{z^{t'}, |t'-t| > w\}$ (where $w$ is a hyperparameter specifying the positive window size). Intuitively, $z^t$ should be closer to the positive set embeddings and further from the negative set embeddings measured by a similarity function $s(z^{t}, z^{t'})$. Using the contrastive INFO-NCE~\cite{Oord2018RepresentationLW} learning objective, we can define $\mathcal{L}_{time}(\phi) = -\sum\limits_{z^{+} \in \mathbf{z^{+}}} \frac{\text{exp}(s(z^{t}, z^{+})/\tau)}{\text{exp}(s(z^{t}, z^{+})/\tau)+\sum_{z^{-}\in \mathbf{z^{-}}}{\text{exp}(s(z^{t}, z^{-})/\tau)}}$, with temperature parameter $\tau$.

% to group image frames close to each other within a video sequence. 

\textbf{Visual Alignment.} We utilize SwAV~\cite{caron2020unsupervised}, a self-supervised learning algorithm to cluster images based on visual features. The algorithm learns a set of $K$ learnable \textit{prototype} vectors, $\mathbf{c} = \{c^{1}, c^{2}, \dots, c^{K}\}$ that are matched with individual images. For training these representations, an image is first augmented in two different ways producing different embeddings $z^{1}$ and $z^{2}$. Then, each embedding's soft assignment to the $K$ prototypes is computed using the Sinkhorn-Knopp algorithm to produce \textit{codes}, $q^{1}$ and $q^{2}$, $K$ dimensional assignment probabilities to each prototype. The SwAV loss function leverages that both embeddings, only differentiated by augmentations, should map to the same codes. The loss function $\mathcal{L}_{vis}(\phi, \mathbf{c}) = l_{swav}(z^{1}, q^{2})+l_{swav}(z^{2}, q^{1})$, updates both the video encoder as well as the prototype set. We refer the reader to the original paper for more details. As used by XSkill~\cite{xu2023xskill},  we map demonstrator and robot images to the same set of prototypes using this loss function, where batches only consist of images from one embodiment.  In our experiments, we show that this way of learning representations maps robot and demonstrator tasks to the same embedding space, \textit{but only when their object movements are similar}.

\vspace{-12mm}
\subsection{Model Architecture Details \label{sec:model_arch}}
\vspace{-12mm}
\textbf{Video Encoding} 

The video encoder $\phi$ is modeled by a CNN-based vision backbone and transformer encoder. $\phi$ individually extracts embeddings for each frame in a demonstration video, where in practice each frame is represented by a 1-timestep sliding window of 8 neighboring images passed into the network to produce a 256-dimensional flattened vision feature vector. At train time, we perform random image augmentations to compute a self-supervised loss~\cite{caron2020unsupervised} and use $K=128$ learnable prototype vectors implemented as a linear layer with no bias as described in Section~\ref{sec:rep_align}.

\textbf{Policy Structure}

The policy $\pi$ consists of two components: a Skill Alignment Transformer (SAT) (introduced by \cite{xu2023xskill}) to model $p(z_{t+1} | s_t, \mathbf{z_R})$, which allows the policy to extract $z_{t+1}$, the next task embedding induced by progressing in the tasks, based on the robot state $s_t$ and prompt video $\mathbf{z_R}$. The second component is a task-conditioned policy $\pi(a_t | s_t, z_{t+1})$, which essentially serves as an inverse dynamics model to decode the robot's current state $s_t$ and the next task embedding $z_{t+1}$ (predicted by SAT) into the correct action. The policy is modeled by Diffusion Policy~\cite{chi2023diffusion}.

\textbf{Hyperparameters}

We borrow hyperparameters from prior works~\cite{caron2020unsupervised, xu2023xskill} for Temporal Alignment and Visual Alignment (Section~\ref{sec:rep_align}), and present hyperparameters for our retrieval algorithm \textsc{Imagine-Demo} (Alg. 2), as well as the optional hyperparameters for fine-tuning the visual representation space (Section 4.2).

\begin{minipage}[h]{0.50\textwidth}
\vspace{-1mm}

{
\begin{tabular}{ll}
\toprule

\textsc{Imagine-Demo} Hyperparam. $\downarrow$ & Value\\
\midrule
OT similarity temperature             & 0.05 \\
TCC similarity temperature            & 0.1 \\
\midrule

Policy $\pi$ Hyperparam.~\cite{chi2023diffusion}$\downarrow$ & Value \\
\midrule
Observation Horizon            & 2   \\
Action Horizon                 & 2    \\
Action Pred. Horizon            & 16   \\
State - Vision Feature Dim.        & 64     \\
State - Proprio. Feature Dim.           & 9 \\
Action Dim.           & 9 \\
Batch Size                 & 128    \\
Training iteration         & 200   \\
Learning rate              & 1e-4  \\
Weight decay              & 1e-6  \\
Optimizer                 & ADAM  \\ 
\bottomrule
\end{tabular}%
}
\label{tab:sim_hyper}

\end{minipage}
\hfill % This will create space between the two minipages
\begin{minipage}[h]{0.48\textwidth}
\vspace{-1mm}

{
\begin{tabular}{ll}
\toprule
Video Encoder $\phi$ Hyperparam.~\cite{xu2023xskill} $\downarrow$ & Value\\
\midrule
Video Clip length   $l$       & 8     \\
Sampling Frames  $T$           & 100   \\
Sinkhorn iterations        & 3     \\
Sinkhorn epsilon           & 0.03  \\
Prototype loss coef        & 0.5   \\
Prototype loss temperature & 0.1   \\
TCN loss coef & 1     \\
TCN positive window  $w_p$      & 4     \\
TCN negative window  $w_n$      & 12    \\
TCN negative samples       & 16    \\
TCN temperature   $\tau_{\text{tcn}}$         & 0.1   \\
Batch Size                 & 28    \\
Training iteration         & 100   \\
Learning rate              & 1e-4  \\
Optimizer                 & ADAM  \\ 
\bottomrule
\end{tabular}%
}
\label{tab:sim_hyper}

\end{minipage}
